# Supplementary material for: Variationality of conformal geodesics in dimension 3
Source: arXiv:2412.04890 ancillary file (2025-08-15)
Supplement: Supplementary file 1 [file KMS-2024-Lagrangian_vanish_CGE.pdf]

```
> with(DifferentialGeometry) : with(Tensor) : with(JetCalculus) : with(GroupActions) :
  with(Tools) : with(LieAlgebras) : with(PDETools) : with(LinearAlgebra) :
  Preferences("ShowFramePrompt",false) :
```

14.10.2024

The purpose of this file is to show that the Euler--Lagrange equations are third-order and that these vanish after substituting the conformal geodesic equations (together with constraints).

We generate conformal geodesic equations in terms of x-vars and their derivatives.

```
> CGE := proc(g)
  local u, acc, orth, del1dot, del2dot, del3dot, xdoteqn, udot, udoteqn, adot, adoteqn, unormsq,
    anormsq, usq, asq, ulist, alist, ueq, aeq, adoteq, i, confgeodeqn, P, C, deldotlist, cge :
```

#### *Defining the relevant objects*

```
u := evalDG(u1[ ] D_x1 + u2[ ] D_x2 + u3[ ] D_x3) :
  # velocity in terms of coordinate frame
acc := evalDG(a1[ ] D_x1 + a2[ ] D_x2 + a3[ ] D_x3) :
  # acceleration in terms of coordinate frame
unormsq := evalDG(ContractIndices(evalDG(g &t u &t u), [[1, 3], [2, 4]]), ) :
  # g(u,u), i.e. square norm of velocity
anormsq := evalDG(ContractIndices(evalDG(g &t acc &t acc), [[1, 3], [2, 4]]), ) :
  # g(a,a), i.e. square norm of acceleration
orth := evalDG(ContractIndices(evalDG(g &t u &t acc), [[1, 3], [2, 4]]), ) :
  # g(u,a), i.e. inner product of velocity and acceleration
P := evalDG(SchoutenTensor(g)) : # Schouten tensor.
C := Christoffel(g) : # Connection of metric g.
```

```
del1dot := DirectionalCovariantDerivative(u, D_x1, C); del2dot :=
  DirectionalCovariantDerivative(u, D_x2, C); del3dot := DirectionalCovariantDerivative(u,
  D_x3, C) :
  # del_1dot := nabla_u(del_x1), del2dot := nabla_u(del_x2), del3dot := nabla_u(del_x3)
deldotlist := [del1dot, del2dot, del3dot] :
ulist := [u1[ ], u2[ ], u3[ ]]: alist := [a1[ ], a2[ ], a3[ ]]:
```

#### *Computing the conformal geodesic equations*

```
xdoteqn := [x1[1] = u1[ ], x2[1] = u2[ ], x3[1] = u3[ ]]: ## x(1) in terms of u
udot := eval(evalDG(convert(u1[1] D_x1 + u2[1] D_x2 + u3[1] D_x3, DGtensor)
  + convert(add((evalDG(ulist[i] deldotlist[i])), i = 1..3), DGtensor)), [x1 = x1[ ], x2
  = x2[ ], x3 = x3[ ]]) : # vector field a = nabla_u(u)
udoteqn := eval(eval(eliminate(DGinfo(evalDG(convert(udot, DGtensor) - convert(acc,
  DGtensor)), "CoefficientSet"), [u1[1], u2[1], u3[1]])[1], ), ) : # u(1) in x, u, a

adot := eval(eval(evalDG(convert(a1[1] D_x1 + a2[1] D_x2 + a3[1] D_x3, DGtensor)
  + convert(add((evalDG(alist[i] deldotlist[i])), i = 1..3), DGtensor)), ), [x1 = x1[ ], x2
  = x2[ ], x3 = x3[ ]]) : # vector field adot = nabla_u(a)
```

```

confgeodeqn := eval(evalDG(convert(-( anormsq + ContractIndices(evalDG(P &t u &t u ),
  [[1, 3], [2, 4]])) u, DGtensor)
+ convert(evalDG(ContractIndices(evalDG(RaiseLowerIndices(InverseMetric(g), P,
  [2])) &t u ), [[1, 3]]), DGtensor )), [x1 = x1[ ], x2 = x2[ ], x3 = x3[ ]]) :
# RHS conformal geodesic equations
adoteqn := eval(eval(eliminate(DGinfo(evalDG(convert(adot , DGtensor)
- convert(confgeodeqn , DGtensor)), "CoefficientSet"), [a1[1], a2[1], a3[1]])[1], ), ) :
### a(1) in terms of x, u, a through conf. geod. eqn.

```

#### Converting quantities from  $x, u, a, a^{(1)}$  variables to  $x, x^{(1)}, x^{(2)}, x^{(3)}$  variables :

```

DGsetup([t], [x1, x2, x3, u1, u2, u3, a1, a2, a3], E, 3) :
ueq := {u1[ ] = x1[1], u2[ ] = x2[1], u3[ ] = x3[1]} union {u1[1] = x1[1, 1], u2[1] = x2[1,
  1], u3[1] = x3[1, 1]} union {u1[1, 1] = x1[1, 1, 1], u2[1, 1] = x2[1, 1, 1], u3[1, 1]
  = x3[1, 1, 1]} : # u in terms of x, x(1)
aeq := eval(eliminate(udoteqn, [a1[ ], a2[ ], a3[ ]])[1], ueq) : ## a in terms of x, x(1), x(2)
adoteq := eval(ueq union aeq union {seq(TotalDiff(aeq[i], t), i = 1..3)}, ) : ## a(1), a, u(1),
  u in terms of x, x(1), x(2), x(3)
cge := eval(eliminate(eval(adoteqn, adoteq), [x1[1, 1, 1], x2[1, 1, 1], x3[1, 1, 1]])[1], [ ] ) :
## expressing x(3) in terms of x, x(1), x(2) through conformal geodesic equations

usq := eval(eval(unormsq, [x1 = x1[ ], x2 = x2[ ], x3 = x3[ ]]), adoteq) : ##g(u, u)
  in terms of x, x(1)
asq := eval(eval(anormsq, [x1 = x1[ ], x2 = x2[ ], x3 = x3[ ]]), adoteq) : ##g(a, a)
  in terms of x, x(1), x(2)
orth := eval(eval(orth, [x1 = x1[ ], x2 = x2[ ], x3 = x3[ ]]), adoteq) :
##g(u, a) in terms of x, x(1), x(2)

DGsetup([x1, x2, x3], N) :
return(cge, adoteq, usq, asq, orth, u, acc , adot, confgeodeqn) :
end proc:

```

### Three-Dimensional Metric (may always be written in diagonal form)

```

> DGsetup([x1, x2, x3], N) :
> g := evalDG(g1(x1, x2, x3) dx1 &t dx1 + g2(x1, x2, x3) dx2 &t dx2 + g3(x1, x2, x3) dx3
  &t dx3 )
  g := g1(x1, x2, x3) dx1 dx1 + g2(x1, x2, x3) dx2 dx2 + g3(x1, x2, x3) dx3 dx3 (1)

```

### Defining conformal geodesic equations:

```

> CGEq := CGE(g) :
> cge := CGEq[1] :
> guu := simplify(CGEq[3]) : gaa := simplify(CGEq[4]) : gua := simplify(CGEq[5]) :
  # g(u, u), g(a, a), g(u, a) respectively

```

### Computing the Riemannian volume form and its value on the triple (u, a, ∇<sub>u</sub>(a))

```

> gM := Matrix([[g1(x1[ ], x2[ ], x3[ ]), 0, 0], [0, g2(x1[ ], x2[ ], x3[ ]), 0], [0, 0, g3(x1[ ],

```

$x2[ ], x3[ ] ] ) : gdet := simplify(Determinant(gM), trig) \# \text{needed for volume form } vol\_g$   
 $gdet := g1(x1[ ], x2[ ], x3[ ]) g2(x1[ ], x2[ ], x3[ ]) g3(x1[ ], x2[ ], x3[ ]) \quad (2)$

>  $u, acc, adot := CGEq[6], CGEq[7], CGEq[8] : \# u, a, \nabla_u(a)$   
 >  $volg := eval(ContractIndices( evalDG( evalDG( convert( evalDG( sqrt(gdet) dx1 \&w dx2 \&w dx3 ), DGtensor ) \&t evalDG(u \&t acc \&t adot) ) ), [[1, 4], [2, 5], [3, 6]] ), [ ] ) :$   
 $\# \# vol\_g(u, a, nabla\_u(a)) \text{ in terms of } x, u, a, a^{(1)}$   
 >  $volg2 := eval(volg, CGEq[2]) : \# vol\_g(u, a, nabla\_u(a)) \text{ in terms of } x, x^{(1)}, x^{(2)}, x^{(3)}$

## Defining Lagrangian

>  $DGsetup([t], [x1, x2, x3], E, 3) :$   
 >  $L := simplify\left(\frac{\sqrt{guu} \cdot volg2}{(guu gaa - gua^2)}, \right) :$

## Defining jet variables:

>  $vars0 := x1[ ], x2[ ], x3[ ] : vars1 := x1[1], x2[1], x3[1] : vars2 := x1[1, 1], x2[1, 1], x3[1, 1] :$   
 $vars3 := x1[1, 1, 1], x2[1, 1, 1], x3[1, 1, 1] : vars4 := x1[1, 1, 1, 1], x2[1, 1, 1, 1],$   
 $x3[1, 1, 1, 1] : vars5 := x1[1, 1, 1, 1, 1], x2[1, 1, 1, 1, 1], x3[1, 1, 1, 1, 1] : vars6 := x1[1,$   
 $1, 1, 1, 1, 1], x2[1, 1, 1, 1, 1, 1], x3[1, 1, 1, 1, 1, 1] :$

## Truncated total derivative

>  $trD := f \rightarrow add(vars1[i] diff(f, vars0[i]) , i = 1 ..3) + add(vars2[i] diff(f, vars1[i]) , i = 1 ..3) + add(vars3[i] diff(f, vars2[i]) , i = 1 ..3) :$

## Total derivative

>  $Der := f \rightarrow add(vars1[i] diff(f, vars0[i]) , i = 1 ..3) + add(vars2[i] diff(f, vars1[i]) , i = 1 ..3) + add(vars3[i] diff(f, vars2[i]) , i = 1 ..3) + add(vars4[i] diff(f, vars3[i]) , i = 1 ..3) + add(vars5[i] diff(f, vars4[i]) , i = 1 ..3) + add(vars6[i] diff(f, vars5[i]) , i = 1 ..3) :$

## Defining (truncated) Euler--Lagrange operator wrt the first coordinate

>  $EL1 := f \rightarrow diff(f, vars0[1]) - trD(diff(f, vars1[1])) + trD(trD(diff(f, vars2[1]))) - trD(trD(trD(diff(f, vars3[1]))) ) :$   
 >  $EL2 := f \rightarrow diff(f, vars0[2]) - trD(diff(f, vars1[2])) + trD(trD(diff(f, vars2[2]))) - trD(trD(trD(diff(f, vars3[2]))) ) :$   
 >  $EL3 := f \rightarrow diff(f, vars0[3]) - trD(diff(f, vars1[3])) + trD(trD(diff(f, vars2[3]))) - trD(trD(trD(diff(f, vars3[3]))) ) :$

## Defining Euler--Lagrange operators (purpose is to check that fourth and fifth order coefficients vanish):

>  $EL1full := f \rightarrow diff(f, vars0[1]) - Der(diff(f, vars1[1])) + Der(Der(diff(f, vars2[1]))) - Der(Der(Der(diff(f, vars3[1]))) ) + Der(Der(Der(Der(diff(f, vars4[1]))))) - Der(Der(Der(Der(Der(diff(f, vars5[1])))))) + Der(Der(Der(Der(Der(Der(diff(f, vars6[1])))))))) :$   
 >  $EL2full := f \rightarrow diff(f, vars0[2]) - Der(diff(f, vars1[2])) + Der(Der(diff(f, vars2[2])))$

$- \text{Der}(\text{Der}(\text{Der}(\text{diff}(f, \text{vars3}[2]))) + \text{Der}(\text{Der}(\text{Der}(\text{Der}(\text{diff}(f, \text{vars4}[2])))))$   
 $- \text{Der}(\text{Der}(\text{Der}(\text{Der}(\text{Der}(\text{diff}(f, \text{vars5}[2])))))$   
 $+ \text{Der}(\text{Der}(\text{Der}(\text{Der}(\text{Der}(\text{Der}(\text{diff}(f, \text{vars6}[2])))))) :$

$> \text{EL3full} := f \rightarrow \text{diff}(f, \text{vars0}[3]) - \text{Der}(\text{diff}(f, \text{vars1}[3])) + \text{Der}(\text{Der}(\text{diff}(f, \text{vars2}[3])))$   
 $- \text{Der}(\text{Der}(\text{Der}(\text{Der}(\text{Der}(\text{diff}(f, \text{vars3}[3]))))) + \text{Der}(\text{Der}(\text{Der}(\text{Der}(\text{diff}(f, \text{vars4}[3])))))$   
 $- \text{Der}(\text{Der}(\text{Der}(\text{Der}(\text{Der}(\text{diff}(f, \text{vars5}[3])))))$   
 $+ \text{Der}(\text{Der}(\text{Der}(\text{Der}(\text{Der}(\text{Der}(\text{diff}(f, \text{vars6}[3])))))) :$

**We show that the Euler--Lagrange equations vanish after substituting. This is enough by symmetry of the indices (diagonal metric).**

$> \text{el1} := \text{EL1}(L) :$

$> \text{EL1sub} := \text{eval}(\text{el1}, \text{cge}) :$

$> \text{EL1subnew} := \text{eval}(\text{EL1sub}, [x1[1] = 1, x2[1] = 0, x3[1] = 0, x1[1, 1] = 0, x2[1, 1] = a, x3[1, 1] = 0]) :$

$> \text{simplify}(\text{EL1subnew})$

0

(3)

$> \text{el2} := \text{EL2}(L) :$

$> \text{EL2sub} := \text{eval}(\text{el2}, \text{cge}) :$

$> \text{EL2subnew} := \text{eval}(\text{EL2sub}, [x1[1] = 1, x2[1] = 0, x3[1] = 0, x1[1, 1] = 0, x2[1, 1] = a, x3[1, 1] = 0]) :$

$> \text{eq2} := \text{simplify}(\text{EL2subnew})$

$\text{eq2} := - \left( -2 g1(x1[ ], x2[ ], x3[ ]) g2(x1[ ], x2[ ], x3[ ]) g3(x1[ ], x2[ ], x3[ ]) (g1(x1[ ], x2[ ], x3[ ]) - 1) \right. \quad (4)$

$$\begin{aligned}
 & \left( \frac{\partial^2}{\partial x1[ ] \partial x3[ ]} g2(x1[ ], x2[ ], x3[ ]) \right) + \left( -3 g2(x1[ ], x2[ ], x3[ ]) \left( \frac{\partial}{\partial x1[ ]} g1(x1[ ], x2[ ], x3[ ]) \right) + \left( \frac{\partial}{\partial x1[ ]} g2(x1[ ], x2[ ], x3[ ]) \right) (g1(x1[ ], x2[ ], x3[ ]) - 1) \right) \\
 & \left( \frac{\partial}{\partial x3[ ]} g1(x1[ ], x2[ ], x3[ ]) \right) + \left( \frac{\partial}{\partial x1[ ]} g2(x1[ ], x2[ ], x3[ ]) \right) (g1(x1[ ], x2[ ], x3[ ]) - 1) \left( \frac{\partial}{\partial x3[ ]} g1(x1[ ], x2[ ], x3[ ]) \right) \\
 & + \left( \frac{\partial}{\partial x3[ ]} g2(x1[ ], x2[ ], x3[ ]) \right) g1(x1[ ], x2[ ], x3[ ]) (g1(x1[ ], x2[ ], x3[ ]) - 1) \left( g3(x1[ ], x2[ ], x3[ ]) \left( \frac{\partial}{\partial x1[ ]} g2(x1[ ], x2[ ], x3[ ]) \right) + \left( \frac{\partial}{\partial x1[ ]} g3(x1[ ], x2[ ], x3[ ]) \right) g2(x1[ ], x2[ ], x3[ ]) \right) \\
 & \left. \right) \Bigg/ (4 g1(x1[ ], x2[ ], x3[ ])^3 / \sqrt{g1(x1[ ], x2[ ], x3[ ]) g2(x1[ ], x2[ ], x3[ ]) g3(x1[ ], x2[ ], x3[ ]) g3(x1[ ], x2[ ], x3[ ]) g2(x1[ ], x2[ ], x3[ ])})
 \end{aligned}$$

$> \text{ToJet}(\text{eval}(\text{eq2}, [x1[ ] = x1, x2[ ] = x2, x3[ ] = x3]), \{g1(x1, x2, x3), g2(x1, x2, x3), g3(x1, x2, x3)\}, \text{notation} = \text{jetnumbers})$

$$\begin{aligned}
 & - \frac{1}{4 g1[ ]^3 / \sqrt{g1[ ] g2[ ] g3[ ]} g3[ ] g2[ ]} (-2 g1[ ] g2[ ] g3[ ] (g1[ ] - 1) g2_{1,3} + ( \\
 & -3 g2[ ] g1_1 + g2_1 (g1[ ] - 1) g2[ ] g3[ ] g1_3 + g2_3 g1[ ] (g1[ ] - 1) (g2[ ] g3_1
 \end{aligned} \quad (5)$$

$$+ g^2_1 g^3[ ]))$$

The above expression vanishes in normal coordinates.

$$> \text{eval}(\%, \{g^1[ ] = 1, g^2[ ] = 1, g^3[ ] = 1, g^1[1] = 0, g^2[1] = 0, g^3[1] = 0\})$$

0

(6)

>

$$> \text{el3} := \text{EL3}(L) :$$

$$> \text{EL3sub} := \text{eval}(\text{el3}, \text{cge}) :$$

$$> \text{EL3subnew} := \text{eval}(\text{EL3sub}, [x^1[1] = 1, x^2[1] = 0, x^3[1] = 0, x^1[1, 1] = 0, x^2[1, 1] = a, x^3[1, 1] = 0]) :$$

$$> \text{eq3} := \text{simplify}(\text{EL3subnew})$$

$$\text{eq3} := \left( 3 \left( -\frac{1}{3} \left( g^1(x^1[ ], x^2[ ], x^3[ ]) g^2(x^1[ ], x^2[ ], x^3[ ]) g^3(x^1[ ], x^2[ ], \right. \right. \right. \quad (7)$$

$$\begin{aligned} & x^3[ ]) (g^1(x^1[ ], x^2[ ], x^3[ ]) - 1) \left( \frac{\partial^2}{\partial x^1[ ] \partial x^2[ ]} g^3(x^1[ ], x^2[ ], x^3[ ]) \right) \Bigg) + g^2(x^1[ ], \\ & x^2[ ], x^3[ ]) g^3(x^1[ ], x^2[ ], x^3[ ])^2 \left( g^2(x^1[ ], x^2[ ], x^3[ ]) a \right. \\ & \left. - \frac{\frac{\partial}{\partial x^2[ ]} g^1(x^1[ ], x^2[ ], x^3[ ])}{2} \right) \left( \frac{\partial}{\partial x^1[ ]} g^1(x^1[ ], x^2[ ], x^3[ ]) \right) \\ & + \frac{1}{6} \left( \left( g^2(x^1[ ], x^2[ ], x^3[ ]) \left( \left( \frac{\partial}{\partial x^2[ ]} g^1(x^1[ ], x^2[ ], x^3[ ]) \right) g^3(x^1[ ], x^2[ ], x^3[ ]) \right. \right. \right. \\ & + g^1(x^1[ ], x^2[ ], x^3[ ]) \left( \frac{\partial}{\partial x^2[ ]} g^3(x^1[ ], x^2[ ], x^3[ ]) \right) \Bigg) \left( \frac{\partial}{\partial x^1[ ]} g^3(x^1[ ], x^2[ ], \right. \\ & x^3[ ]) \Bigg) + g^1(x^1[ ], x^2[ ], x^3[ ]) \left( \frac{\partial}{\partial x^2[ ]} g^3(x^1[ ], x^2[ ], x^3[ ]) \right) \left( \frac{\partial}{\partial x^1[ ]} g^2(x^1[ ], x^2[ ], \right. \\ & x^3[ ]) \Bigg) g^3(x^1[ ], x^2[ ], x^3[ ]) \Bigg) (g^1(x^1[ ], x^2[ ], x^3[ ]) - 1) \Bigg) \Bigg) / (2 g^1(x^1[ ], \\ & x^2[ ], x^3[ ])^3 / \\ & \sqrt[2]{g^1(x^1[ ], x^2[ ], x^3[ ]) g^2(x^1[ ], x^2[ ], x^3[ ]) g^3(x^1[ ], x^2[ ], x^3[ ]) g^2(x^1[ ], x^2[ ], \\ & x^3[ ]) g^3(x^1[ ], x^2[ ], x^3[ ])} \end{aligned}$$

$$> \text{ToJet}(\text{eval}(\text{eq3}, [x^1[ ] = x^1, x^2[ ] = x^2, x^3[ ] = x^3]), \{g^1(x^1, x^2, x^3), g^2(x^1, x^2, x^3), g^3(x^1, x^2, x^3)\}, \text{notation} = \text{jetnumbers})$$

$$\frac{1}{2 g^1[ ]^3 \sqrt[2]{g^1[ ] g^2[ ] g^3[ ]} g^2[ ] g^3[ ]} \left( 3 \left( -\frac{g^1[ ] g^2[ ] g^3[ ] (g^1[ ] - 1) g^3_{1,2}}{3} \right. \right. \quad (8)$$

$$\left. \left. + g^2[ ] g^3[ ]^2 \left( g^2[ ] a - \frac{g^1_2}{2} \right) g^1_1 \right) \right)$$

$$+ \frac{(g^2[ ] (g^1[ ] g^3_2 + g^1_2 g^3[ ]) g^3_1 + g^1[ ] g^3_2 g^2_1 g^3[ ]) (g^1[ ] - 1)}{6} \Bigg)$$

**Vanishes in normal coordinates.**

$$> \text{eval}(\%, \{g^1[ ] = 1, g^2[ ] = 1, g^3[ ] = 1, g^1[1] = 0, g^2[1] = 0, g^3[1] = 0\})$$

0

(9)

>

**We also check that the fourth and fifth order coefficients of the Euler--Lagrange equations vanish, i.e., that  $\text{ord}(\text{EL}) = 3$ .**

>

$$> \text{ellfull} := \text{EL1full}(L) : \text{el2full} := \text{EL2full}(L) : \text{el3full} := \text{EL3full}(L) :$$

>

**Vanishing of fifth order coefficients:**

$$> \text{diff}(\text{ellfull}, x1[1, 1, 1, 1, 1]);$$

0

(10)

$$> \text{simplify}(\text{diff}(\text{ellfull}, x2[1, 1, 1, 1, 1]), [\text{guu} - 1, \text{gua}])$$

0

(11)

$$> \text{simplify}(\text{diff}(\text{ellfull}, x3[1, 1, 1, 1, 1]), [\text{guu} - 1, \text{gua}])$$

0

(12)

>

**Vanishing of fourth order coefficients:**

$$> \text{simplify}(\text{diff}(\text{ellfull}, x1[1, 1, 1, 1]), [\text{guu} - 1, \text{gua}]);$$

0

(13)

$$> \text{simplify}(\text{diff}(\text{ellfull}, x2[1, 1, 1, 1]), [\text{guu} - 1, \text{gua}])$$

0

(14)

$$> \text{simplify}(\text{diff}(\text{ellfull}, x3[1, 1, 1, 1]), [\text{guu} - 1, \text{gua}])$$

0

(15)

**We check that the EL equations are linear in third-order derivatives**

>

$$> \text{degree}(\text{ell}, x1[1, 1, 1])$$

# degree command indicates cubic degree, but perhaps there are simplifications

3

(16)

**We make use of the coeff-command:**

$$> \text{coeff}(a^3 + a^2 + a + b, a^2)$$

1

(17)

$$> \text{simplify}(\text{coeff}(\text{ell}, x1[1, 1, 1, 1]^3), [\text{guu} - 1, \text{gua}])$$

0

(18)

$$> \text{simplify}(\text{coeff}(\text{ell}, x1[1, 1, 1, 1]^2), [\text{guu} - 1, \text{gua}])$$

0

(19)

$$> \text{simplify}(\text{coeff}(\text{ell}, x2[1, 1, 1, 1]^3), [\text{guu} - 1, \text{gua}])$$

0

(20)

$$\text{> simplify(coeff(el1, x2[1, 1, 1, 1]^2), [guu - 1, gua])}$$

0

(21)

$$\text{> simplify(coeff(el1, x3[1, 1, 1, 1]^3), [guu - 1, gua])}$$

0

(22)

$$\text{> simplify(coeff(el1, x3[1, 1, 1, 1]^2), [guu - 1, gua])}$$

0

(23)

We conclude that EL is linear in third-order derivatives.

>

**Checking that the rank of EL in 3rd jets is rank 2:**

$$\text{> simplify(eval(ToJet(eval([diff(el1, x1[1, 1, 1]), diff(el1, x2[1, 1, 1]), diff(el1, x3[1, 1, 1])],$$

$$\{x1[1] = 1, x2[1] = 0, x3[1] = 0, x1[1, 1] = 0, x2[1, 1] = a, x3[1, 1] = 0\}), \{g1(x1[1, 1], x2[1, 1], x3[1, 1]), g2(x1[1, 1], x2[1, 1], x3[1, 1]), g3(x1[1, 1], x2[1, 1], x3[1, 1])\}, notation = jetnumbers), \{g1[1, 1] = 1, g2[1, 1] = 1, g3[1, 1] = 1, g1[1] = 0, g2[1] = 0, g3[1] = 0\}))$$

[0, 0, 0]

(24)

$$\text{> simplify(eval(ToJet(eval([diff(el2, x1[1, 1, 1]), diff(el2, x2[1, 1, 1]), diff(el2, x3[1, 1, 1])],$$

$$\{x1[1] = 1, x2[1] = 0, x3[1] = 0, x1[1, 1] = 0, x2[1, 1] = a, x3[1, 1] = 0\}), \{g1(x1[1, 1], x2[1, 1], x3[1, 1]), g2(x1[1, 1], x2[1, 1], x3[1, 1]), g3(x1[1, 1], x2[1, 1], x3[1, 1])\}, notation = jetnumbers), \{g1[1, 1] = 1, g2[1, 1] = 1, g3[1, 1] = 1, g1[1] = 0, g2[1] = 0, g3[1] = 0\}))$$

[0, 0, 1]

(25)

$$\text{> simplify(eval(ToJet(eval([diff(el3, x1[1, 1, 1]), diff(el3, x2[1, 1, 1]), diff(el3, x3[1, 1, 1])],$$

$$\{x1[1] = 1, x2[1] = 0, x3[1] = 0, x1[1, 1] = 0, x2[1, 1] = a, x3[1, 1] = 0\}), \{g1(x1[1, 1], x2[1, 1], x3[1, 1]), g2(x1[1, 1], x2[1, 1], x3[1, 1]), g3(x1[1, 1], x2[1, 1], x3[1, 1])\}, notation = jetnumbers), \{g1[1, 1] = 1, g2[1, 1] = 1, g3[1, 1] = 1, g1[1] = 0, g2[1] = 0, g3[1] = 0\}))$$

[0, -1, 0]

(26)

>

**Finally here is a simple check of the transformation rule for the Lagrangian (in geodesic coordinates and normalized frame)**

**Notations**  $u = \dot{x}$ ,  $a = \ddot{x}$ ,  $b = \ddot{\ddot{x}}$ ,  $f = \nabla \phi$ ,  $h = \dot{f}$

$$\text{> } U := [seq(u[i], i = 1..3)] : A := [seq(a[i], i = 1..3)] : B := [seq(b[i], i = 1..3)] : F := [seq(f[i], i = 1..3)] : H := [seq(h[i], i = 1..3)] :$$

$$uu := add(U[i] \cdot U[i], i = 1..3) : ua := add(U[i] \cdot A[i], i = 1..3) : uf := add(U[i] \cdot F[i], i = 1..3) :$$

$$Ac := [seq(a[i] - uf U[i] + f, i = 1..3)] : Bc := [seq(B[i] + uf F[i] + H[i], i = 1..3)] :$$

$$aa := add(A[i] \cdot A[i], i = 1..3) : aca := add(A[i] \cdot Ac[i], i = 1..3) : acac := add(Ac[i] \cdot Ac[i], i = 1..3) :$$

$$\text{> } V := Determinant(Matrix([U, A, B])) : Vc := Determinant(Matrix([U, Ac, Bc])) :$$

$$S := \arccos\left(\frac{aca}{\sqrt{aa} \cdot \sqrt{acac}}\right) : L := \frac{V}{aa} : Lc := \frac{Vc}{acac} :$$

$$\text{> } TD := f \rightarrow add(diff(f, U[i]) A[i] + diff(f, A[i]) B[i] + diff(f, F[i]) H[i], i = 1..3) :$$

$$\text{> simplify(eval(Lc - L - TD(S), \{u1 = 1, u2 = 0, u3 = 0, a1 = 0, a2 = a, a3 = 0\}), symbolic)}$$

0

(27)

>
